# Supplementary material for: Montague semantics and modifier consistency measurement in neural language models
Source: arXiv:2212.04310 source file (2024-12-18)
Supplement: Supplementary file 1 [file appendix_extra.tex]

\section{Extra Metamorphic Relations (Intersectivity Index?)} \label{sec:apd_extra_relations}

\textbf{Objectives:}
\begin{itemize}
    \item explicit comparison between two adjectives;
    \item relative measurement to cancel the noise;
    \item treat adjectives as transformations (never look at their embeddings in isolation).
\end{itemize}

\textbf{Example:} $d(\text{``Canadian writer''}, \text{``Canadian surgeon''})<d(\text{``skilful writer''}, \text{``skilful surgeon''})$

\textbf{Intuition.} ``Canadian'' is an intersective adjective whereas ``skilful'' is not. As a result, we expect ``Canadian + noun1'' to have something in common with ``Canadian + noun2'', i.e. the fact that they are both Canadian. In contrast, ``skilful + noun1'' and ``skilful + noun2'' are similar if and only if the two nouns are already similar.

Formalization of the metamorphic relation:
\begin{itemize}
    \item \textbf{Input A.} Two arbitrary nouns (or longer phrases) $N_i, N_j$.
    \item \textbf{Input B.} Two adjectives $A,B$ that we want to compare.
    \item \textbf{Output.} Whether the following is true
    \begin{equation}
    \label{eq:extra_meta}
        d(A+N_i,A+N_j)<d(B+N_i,B+N_j)
    \end{equation}
    where $+$ represents concatenation.
\end{itemize}

\textbf{Usage (1): comparing different adjective categories.} Compute the average veracity of Equation \ref{eq:extra_meta} where $A\in\mathcal{A}$ and $B\in\mathcal{B}$ are any adjectives in the categories $\mathcal{A}$ (e.g. intersective) and $\mathcal{B}$ (e.g. ambiguous). In contrast, the pair of nouns (or longer phrases) $N_i\in\mathcal{N}$ and $N_j\in\mathcal{N}$ can be extracted from the same set $\mathcal{N}$ as long as $N_i\neq N_j$, since Equation \ref{eq:extra_meta} should yield equality for $N_i= N_j$. We expect the average veracity to be higher when $\mathcal{A}$ is the intersective category. How do other categories compare?

\textbf{Usage (2): comparing individual adjective pairs.} In the same way as usage (1), average over any $N_i\in\mathcal{N}$ and $N_j\in\mathcal{N}$. However, compute the average veracity for two specific adjectives $A\in\mathcal{C}$ and $B\in\mathcal{C}$, where $\mathcal{C}$ is the union of all adjective categories. If we do this for all possible pairs $(A,B)$, we end up having an empirical measure for the intersectivity of each adjective. That is, an adjective $A$ that ``wins'' most pairings $(A,B)$ is relatively more intersective than the rest of the set $\mathcal{C}$. An ``intersectivity ranking'' of the adjectives in $\mathcal{C}$ might reveal interesting patterns. Note that with usage (2) we do not need a ground-truth on the category of each adjective (truly metamorphic!).

\begin{table}[h!]
    \centering
    \begin{tabular}{@{}llllllllll@{}}
    \toprule
    \multicolumn{1}{c}{\textbf{Models}} & \multicolumn{9}{c}{\textbf{Adjective Type Pair}}                                                                                                                                                                                                                                                                                                                                                                                                                                                                                               \\ \midrule
    \multicolumn{1}{c}{\textbf{}}       & \begin{tabular}[c]{@{}l@{}}(S-I,\\ S-I)\end{tabular}      & \begin{tabular}[c]{@{}l@{}}(S-I,\\ S-NI)\end{tabular}   & \begin{tabular}[c]{@{}l@{}}(S-I, \\ NS-Pl)\end{tabular}  & \begin{tabular}[c]{@{}l@{}}(S-I, \\ NS-Pr)\end{tabular}  & \begin{tabular}[c]{@{}l@{}}(S-I,\\ A)\end{tabular}        & \begin{tabular}[c]{@{}l@{}}(S-NI, \\ S-NI)\end{tabular} & \begin{tabular}[c]{@{}l@{}}(S-NI, \\ NS-Pl)\end{tabular} & \begin{tabular}[c]{@{}l@{}}(S-NI,\\ NS-Pr)\end{tabular} & \begin{tabular}[c]{@{}l@{}}(S-NI, \\ A)\end{tabular}  \\ \midrule
    BERT                                & 0.4842                                                    & 0.7961                                                  & 0.7777                                                   & 0.8146                                                   & 0.6198                                                    & 0.4909                                                  & 0.5533                                                   & 0.5508                                                  & 0.2676                                                    \\
    DistilRoBERTa                       & 0.4628                                                    & 0.7217                                                  & 0.6813                                                   & 0.5537                                                   & 0.7052                                                    & 0.5090                                                  & 0.4500                                                   & 0.3246                                                  & 0.4292                                                    \\
    T5                                  & 0.4347                                                    & 0.6528                                                  & 0.6391                                                   & 0.5602                                                   & 0.6832                                                    & 0.3151                                                  & 0.4337                                                   & 0.3874                                                  & 0.4696                                                    \\
    DPR                                 & 0.4727                                                    & 0.3719                                                  & 0.3954                                                   & 0.4616                                                   & 0.6584                                                    & 0.4787                                                  & 0.5117                                                   & 0.5844                                                  & 0.7474                                                    \\
    LaBSE                               & 0.6165                                                    & 0.4435                                                  & 0.3752                                                   & 0.5354                                                   & 0.3278                                                    & 0.2727                                                  & 0.4186                                                   & 0.6266                                                  & 0.3585                                                    \\
    MiniLM                              & 0.4330                                                    & 0.6639                                                  & 0.7554                                                   & 0.5625                                                   & 0.8374                                                    & 0.6000                                                  & 0.5606                                                   & 0.4209                                                  & 0.6616                                                    \\ \midrule
    Glove                               & 0.6082                                                    & 0.6859                                                  & 0.7309                                                   & 0.7095                                                   & 0.4738                                                    & 0.4121                                                  & 0.5516                                                   & 0.5205                                                  & 0.2828                                                    \\
    Word2Vec                            & 0.3785                                                    & 0.7644                                                  & 0.6844                                                   & 0.5147                                                   & 0.9972                                                    & 0.4545                                                  & 0.4371                                                   & 0.2932                                                  & 0.7626                                                    \\ \midrule
                                        & \begin{tabular}[c]{@{}l@{}}(NS-Pl, \\ NS-Pl)\end{tabular}      & \begin{tabular}[c]{@{}l@{}}(NS-Pl, \\ NS-Pr)\end{tabular} & \begin{tabular}[c]{@{}l@{}}(NS-Pl, \\ A)\end{tabular} & \begin{tabular}[c]{@{}l@{}}(NS-Pr,\\ NS-Pr)\end{tabular} & \begin{tabular}[c]{@{}l@{}}(NS-Pr, \\ A)\end{tabular} & \begin{tabular}[c]{@{}l@{}}(A,\\ A)\end{tabular}   \\ \midrule
    BERT                                & 0.4097                                                         & 0.5014                                                    & 0.2693                                                & 0.4605                                                   & 0.2445                                                & 0.6060                                                 \\
    DistilRoBERTa                       & 0.5198                                                         & 0.3732                                                    & 0.4882                                                & 0.5944                                                   & 0.6212                                                & 0.4848                                                 \\
    T5                                  & 0.5281                                                         & 0.4240                                                    & 0.5566                                                & 0.5314                                                   & 0.6255                                                & 0.4848                                                 \\
    DPR                                 & 0.5296                                                         & 0.5668                                                    & 0.7306                                                & 0.4535                                                   & 0.6515                                                & 0.7575                                                 \\
    LaBSE                               & 0.4053                                                         & 0.6741                                                    & 0.4814                                                & 0.5384                                                   & 0.2640                                                & 0.6666                                                 \\
    MiniLM                              & 0.5123                                                         & 0.3407                                                    & 0.5914                                                & 0.4185                                                   & 0.7099                                                & 0.3939                                                 \\ \midrule
    Glove                               & 0.5182                                                         & 0.4644                                                    & 0.2200                                                & 0.6363                                                   & 0.2424                                                & 0.7878                                                 \\
    Word2Vec                            & 0.4457                                                         & 0.3674                                                    & 0.8204                                                & 0.5954                                                   & 0.8636                                                & 0.3030                                                 \\ \bottomrule \\
    \end{tabular}
    \caption{Satisfaction score (consistency) for the set distance property across adjective phrase pairs (Equation~\ref{eq:extra_meta}), for noun phrases with pairs of adjectives of the indicated types (AN format). We use the following shorthand notation in the table columns:
    A: Ambiguous, S-I: Subsective-Intersective, S-NI: Subsective Non-Intersective, NS-Pl: Plain Non-Subsective, NS-Pr: Privative Non-Subsective}
    \label{tab:setdist_pair_an}
    \end{table}
